# Supplementary material for: Don't sweat the small stuff, classify the rest: Sample Shielding to protect text classifiers against adversarial attacks
Source: arXiv:2205.01714 source file (2022-05-03)
Supplement: Supplementary file 1 [file appendix.tex]

\newpage
\onecolumn
\appendix

\newpage
\twocolumn
